# Supplementary material for: A Method For Automated Drone Viewpoints to Support Remote Robot Manipulation
Source: arXiv:2208.04391 source file (2022-08-08)
Supplement: Supplementary file 1 [file 7-appendix.tex]

\appendices
\section{IMPLEMENTATION QUANTITIES} \label{app:quantities}

% \begin{table}[h]
% \centering
%   \caption{Constant values in implementation and optimization. }
%   \label{table:constant}
%   \setlength\tabcolsep{8pt}
%   \begin{tabular}{ll|ll}
%     \toprule
%     \multicolumn{4}{c}{Characterization}\\
%     \cmidrule(r){1-4}
%     \textit{Constant} & \textit{Value} & \textit{Constant} & \textit{Value} \\
%     $\Delta p_x$ & 0.05 m & $\Delta p_z$ & 0.05 m\\
%     $\Delta p_y$ & 0.05 m & robot size & 0.1m\\
%     \midrule
%     \multicolumn{4}{c}{Optimization weights}\\
%     \cmidrule(r){1-4}
%     $w_1$ & 10 & $w_5$ & 1000\\
%     $w_2$ & 5 & $w_6$ & 100\\
%     $w_3$ & 10 & $w_7$ & 300\\
%     $w_4$ & 500 & $w_8$ & 1000\\
%     \midrule
%     \multicolumn{4}{c}{Optimization constants}\\
%     \cmidrule(r){1-4}
%     $f_{fov}$ & 2 & $P$ & 3\\
%     $\theta_{ref} $ & 5$\pi$/4 rad & $\sigma$ & 0.1 m\\
%     \midrule
%     \multicolumn{4}{c}{Alternate view constants}\\
%     \cmidrule(r){1-4}
%     $\epsilon$ & 0.1 & $w_9$ & 1\\
% \bottomrule
%   \end{tabular}
% \end{table}
